# Supplementary material for: Efficiency of Non-Truthful Auctions in Auto-bidding with Budget Constraints
Source: arXiv:2310.09271 source file (2024-04-18)
Supplement: Supplementary file 1 [file appendix.tex]

% \section{Missing proofs}
% \subsection{Proof of Theorem~\ref{thm:fpa_IOPT_ub}}
% \label{app:fpa_iopt}
% \begin{proof}[Proof of Theorem~\ref{thm:fpa_IOPT_ub}]
% We split the bidders into two sets:
% \begin{align*}
% A_B = \{i \in A \text{ } | \text{ } B_i \le \sum_{j \in N(i)} v_{i,j}\} \text{ and }
% A_{\bB} = A \setminus A_B.
% \end{align*}
% Note that, by the definition of liquid welfare, for $i \in A_B$, we have $\LW(i) = B_i \geq \IOPT(i)$.
% Thus, we have
% \begin{equation}
% \label{eq:A_B}
%     \LW(A_B) \ge \IOPT(A_B).
% \end{equation}
% We further split $A_{\bB}$ in to two sets.
% We define $A_{\bB1}$ as the set of bidders $i$ for which there exists at least one query $j \in O(i) \setminus N(i)$ such that if bidder $i$ wins query $j$ as well then their total value would be at least $B_i$.
% % that $i$'s welfare in the equilibrium plus $v_{i,j}$ is at least $B_i$.
% In other words, if bidder $i$ gets this extra query $j$, then they will achieve their optimal liquid welfare $B_i$.
% Next, we define $A_{\bB0} = A_{\bB} \setminus A_{\bB1}$.
% These are the bidders for which we can add any query in $O(i) \setminus N(i)$ and their total value would still be at most $B_i$.
% Formally, the sets are defined as
% \begin{align*}
% A_{\bB1} = \{i \in A_{\bB} \text{ } | \text{ } \exists j \in O(i) \setminus N(i), s.t. \text{ } v_{i,j} + \sum_{j' \in N(i)} v_{i,j'} \ge B_i \} \quad\text{and}\quad A_{\bB0} = A_{\bB} \setminus A_{\bB1}.
% \end{align*}

% We first bound $\IOPT(A_{\bB1})$ and $\IOPT(A_{\bB0})$ in Lemma~\ref{lemma:A_B1} and Lemma~\ref{lemma:A_B0} below, and then put everything together using the constraint that the total spend in the auction is upper bounded by the total liquid welfare.
% \begin{lemma}
% \label{lemma:A_B1}
% We have $\sum_{i \in A_{\bB1}} \sum_{j \in O(i) \setminus N(i)} \Spend(j) + \LW(A_{\bB1}) \ge \IOPT(A_{\bB1})$.
% \end{lemma}
% \begin{proof}
% Fix any bidder $i \in A_{\bB1}$ and consider a query $j' \in O(i) \setminus N(i)$ such that $v_{i,j} + \sum_{j \in N(i)} v_{i,j} \ge B_i$ (such a query $j'$ must exist by definition of $A_{\bB1}$).
% We claim that $\Spend(j') \geq B_i - \sum_{j \in N(i)} v_{i,j}$ in any equilibrium of FPA.
% We will prove this by contradiction, so assume $\Spend(j') < B_i - \sum_{j \in N(i)} v_{i,j}$.
% Then the highest bid on $j'$ must be at most $B_i - \sum_{j \in N(i)} v_{i,j}$.
% Now, observe that if bidder $i$ bids $B_i - \sum_{j \in N(i)} v_{i,j}$ on query $j'$ then bidder $i$ would win query $j'$.
% Their total value would then be $B_i$ and their total spend would be at least $B_i$.
% Thus their value has increased while both their budget and ROS constraints are satisfied.
% This contradicts the assumption that the bidders are in equilibrium.
% % , having a total spend at most $B_i$, and total value at least $B_i$. i.e., bidder $i$ can increase their value while satisfying their constraints, which contradicts the assumption that the bidders are in an equilibrium.
% We conclude that $\Spend(j') \ge B_i - \sum_{j \in N(i)} v_{i,j}$ for all bidders $i \in A_{\bB1}$.
% Using the trivial upper bound $\Spend(j') \leq \sum_{j \in O(i) \setminus N(i)} \Spend(j)$ (since $j' \in O(i) \setminus N(i)$), this implies that $\sum_{j \in O(i) \setminus N(i)} \Spend(j) + \sum_{j \in N(i)} v_{i,j}$ for $i \in A_{\bB1}$.
% We thus have that,
% \begin{align*}
%     \IOPT(A_{\bB1})
%     & \leq \sum_{i \in A_{\bB1}} B_i \\
%     & \leq \sum_{i \in A_{\bB1}} \sum_{j \in O(i) \setminus N(i)} \Spend(j) + \sum_{i \in A_{\bB1}} \sum_{j \in N(i)} v_{i,j} \\
%     & \leq \sum_{i \in A_{\bB1}} \sum_{j \in O(i) \setminus N(i)} \Spend(j) + \LW(A_{\bB1}),
% \end{align*}
% as claimed.
% Note that the first line is because $\IOPT(A_{\bB1}) = \sum_{i \in A_{\bB1}} \min \{ B_i, \sum_{j \in O(i)} v_{i,j}\} \leq \sum_{i \in A_{\bB1}} B_i$.
% \end{proof}

% Summing up for all bidders in $A_{\bB1}$:


% \begin{align*}
%     \sum_{i \in A_{\bB1}} \sum_{j \in O(i) - N(i)} \Spend(j) &\ge \sum_{i \in A_{\bB1}} (B_i - \sum_{j \in N(i)} v_{i,j}) \\
%     \sum_{i \in A_{\bB1}} \sum_{j \in O(i) - N(i)} \Spend(j) + \sum_{i \in A_{\bB1}} \sum_{j \in N(i)} v_{i,j} &\ge \sum_{i \in A_{\bB1}} B_i \\
%     \sum_{i \in A_{\bB1}} \sum_{j \in O(i) - N(i)} \Spend(j) + \LW(A_{\bB1}) &\ge \sum_{i \in A_{\bB1}} B_i \\
%     \sum_{i \in A_{\bB1}} \sum_{j \in O(i) - N(i)} \Spend(j) + \LW(A_{\bB1}) &\ge \IOPT(A_{\bB1})
% \end{align*}


% \end{proof}


% \begin{lemma}
% \label{lemma:A_B0}
% We have $\sum_{i \in A_{\bB0}} \sum_{j \in O(i) \setminus N(i)} \Spend(j) + \LW(A_{\bB0}) \ge \IOPT(A_{\bB0})$.
% \end{lemma}

% \begin{proof}
% %\chrisnote{The proof is similar to the proof of Lemma~\ref{lemma:A_B1}.}
% The proof is similar to the proof of Lemma~\ref{lemma:A_B1}.
% For $i \in A_{\bB0}$, we claim that for each query $j' \in O(i) \setminus N(i)$, $\Spend(j')$ is at least $v_{i,j'}$. Again, we prove this by contradiction. Assume there exists $j' \in O(i) \setminus N(i)$, such that $\Spend(j') < v_{i,j'}$. Then bidder $i$ can bid $v_{i,j'}$ to win query $j'$.
% Note that
% \[
%     c_{i,j'} + \sum_{j \in N(i)} c_{i,j}
%     \leq v_{i,j'} + \sum_{j \in N(i)} c_{i,j}
%     < B_i,
% \]
% where the first inequality uses that bidder $i$ bids and pays $v_{i,j'}$ on query $j'$ and that bidder $i$'s ROS constraint was initially satisfied and the second is by definition of $A_{\bB0}$.
% But this shows that bidder $i$ can improve their value without violating their constraints,
% % By definition of $A_{\bB0}$, it must be $v_{i,j'} + \sum_{j \in N(i)} v_{i,j} < B_i$.
% % Thus, bidder $i$'s budget constraint must 
% % so $i$ would not break their budget constraint $B_i$, and also would not break their value constraint because both their spend and value increase by $v_{i,j}$.
% which contradicts the assumption that the bidders are in an equilibrium. Thus, it must be $\Spend(j') \ge v_{i,j'}$ for all $i \in A_{\bB0}$ and $j' \in O(i) \setminus N(i)$.
% In particular, $\sum_{j \in O(i) \setminus N(i)} \Spend(j) \geq \sum_{j \in O(i) \setminus N(i)} v_{i,j}$.
% Following a similar argument as in Lemma~\ref{lemma:A_B1}, we have that
% \begin{align*}
%     \IOPT(A_{\bB0})
%     & \leq \sum_{i \in A_{\bB0}} \sum_{j \in O(i)} v_{i,j} \\
%     & = \sum_{i \in A_{\bB0}} \sum_{j \in O(i) \setminus N(i)} v_{i,j} + \sum_{i \in A_{\bB0}} \sum_{j \in N(i)} v_{i,j} \\
%     & \leq \sum_{i \in A_{\bB0}} \sum_{j \in O(i) \setminus N(i)} \Spend(j) + \LW(A_{\bB0}).
% \end{align*}
% The first inequality is because $\IOPT(A_{\bB0}) = \sum_{i \in A_{\bB0}} \min \{ B_i, \sum_{j \in O(i)} v_{i,j}\} \leq \sum_{i \in A_{\bB0}} \sum_{j \in O(i)} v_{i,j}$.
% \end{proof}


% % Summing up for all bidders in $A_{\bB0}$:

% % \begin{align*}
% % \sum_{i \in A_{\bB0}} \sum_{j \in O(i) - N(i)} \Spend(j)
% % &\ge \sum_{i \in A_{\bB0}} \sum_{j \in O(i) - N(i)} v_{i,j}   \\
% % \LW(A_{\bB0}) + \sum_{i \in A_{\bB0}} \sum_{j \in O(i) - N(i)} \Spend(j)
% % &\ge \sum_{i \in A_{\bB0}} \sum_{j \in N(i)} v_{i,j} + \sum_{i \in A_{\bB0}} \sum_{j \in O(i) - N(i)} v_{i,j}   \\
% % &\ge \sum_{i \in A_{\bB0}} \sum_{j \in O(i) } v_{i,j} \\
% % &\ge \IOPT(A_{\bB0})
% % \end{align*}

% % The last line holds because $\IOPT(A_{\bB0}) = \sum_{i \in A_{\bB0}} \min \{ B_i, \sum_{j \in O(i)} v_{i,j}\}$.

% % \end{proof}

% % Now we are ready to put everything together. 
% We now return to the proof of Theorem~\ref{thm:fpa_IOPT_ub}.
% Since each bidder's spend is at most their liquid welfare, we have that
% \begin{align*}
%     \LW(A) &\ge \sum_{i \in A} \sum_{j \in O(i)} \Spend(j) \\
%     &\ge \sum_{i \in A_{\bB1}} \sum_{j \in O(i) \setminus N(i)} \Spend(j) 
%     + \sum_{i \in A_{\bB0}} \sum_{j \in O(i) \setminus N(i)} \Spend(j)
% \end{align*}

% Combining Inequality \eqref{eq:A_B}, Lemma~\ref{lemma:A_B1} and Lemma~\ref{lemma:A_B0}, we have
% \begin{align*}
%     \IOPT &= \IOPT(A_B) + \IOPT(A_{\bB1}) + \IOPT(A_{\bB0}) \\
%     &\le \LW(A_B) + \sum_{i \in A_{\bB1}} \sum_{j \in O(i) \setminus N(i)} \Spend(j) + \LW(A_{\bB1})\\
%     &+ \LW(A_{\bB0}) + \sum_{i \in A_{\bB0}} \sum_{j \in O(i) \setminus N(i)} \Spend(j) \\
%     &\le \LW(A_B) + \LW(A_{\bB1}) + \LW(A_{\bB0}) + \LW(A)\\
%     &= 2 \LW(A),
% \end{align*}
% which completes the proof.
% \end{proof}

% \subsection{Proof of Theorem~\ref{thm:rfpa_uniform_ub}}
% \label{app:uniform_rfpa}
% \begin{proof}[Proof of Theorem~\ref{thm:rfpa_uniform_ub}]
% The proof is similar to Theorem~\ref{thm:rfpa_ub}. Case 1 and Case 2 are the same as in Theorem~\ref{thm:rfpa_ub}. For Case 3, we have the following lemma instead of Lemma~\ref{lemma:undominated_bid_lb}:

% \begin{lemma}
% \label{lemma:uniform_undominated_bid_lb}
% Suppose the bidders are assumed to bid uniformly. Fix bidder $i$ and query $j$.
% For any set of undominated bids, if $\pi_{i,j} \in (0, 1)$ and $V_i < B_i$ then $b_{i,j} = v_{i,j}$.
% \end{lemma}
% \begin{proof}
% We denote bidder $i$'s uniform bid multiplier as $m_i$, i.e.~for every query $j \in Q$, $b_{i,j} = m_i \cdot v_{i,j}$. Let $\pi$ be the allocation in equilibrium $\Eq$. It is easy to see that $m_i \le 1$ when $V_i > 0$. Assume the opposite that $m_i > 1$, then we have $b_{i, j} > v_{i, j}$. If there exists $\pi_{i, j} > 0$, then $\sum_{j \in Q} \pi_{i, j}\cdot b_{i, j} > \sum_{j \in Q} \pi_{i, j} \cdot v_{i, j}$, i.e., the ROS constraint is violated.

% Next we show that $m_i \ge 1$. Assume the opposite that $m_i < 1$. Let $\Cost(m)$ be the cost function of bidder $i$'s uniform multiplier and $V(m)$ the the value function of bidder $i$'s uniform multiplier. Note that the ROS constraint is always satisfied as long as $m_i \le 1$. So the only reason why $m_i < 1$ would be that if bidder $i$ deviates to $m = 1$, they may violate their budget constraint i.e.~$B_i < \Cost(1) = V(1)$. In the equilibrium $\Eq$, we have $m_i < 1$, and $\Cost(m_i) < V(m_i) < B_i$ where the last inequality is by the hypothesis of this lemma. Because $\Cost(m)$ and $V(m)$ are both monotone non-decreasing functions, there must exist $m' \in (m_i, 1)$ such that $V(m') > V(m_i)$ and $\Cost(m') < B_i$. This contradicts the fact that bidder $i$ is in an equilibrium. We conclude that $m_i = 1$.
% \end{proof}
% % Thus, Case 3 in this setting:
% \paragraph{Case 3: $0 < \pi_{i,j} < \pis_{i,j} < 1$.}
% Fix a query $j$ and let $\beta_j = b_{i,j} / b_{\oi, j} \in (1/\alpha, \alpha)$.
% Define
% \[
%     m_{\beta} = \frac{1}{2} \ln\left( 1 + \frac{\ln \beta}{\ln \alpha} \right).
% \]
% We have that $\pi_{i,j} = m_{\beta}$.
% Next, by Lemma~\ref{lemma:uniform_undominated_bid_lb}, we have $b_{i,j} \geq v_{i,j}$.
% In particular, we have
% \begin{align*}
% \Spend(j) &= m_{\beta} \cdot b_{i,j} + (1 - m_{\beta}) \cdot b_{\bar{i},j} \\
% &\ge m_{\beta} \cdot v_{i,j} + (1 - m_{\beta}) \cdot \frac{v_{i,j}}{\beta}\\
% & = v_{i,j} \cdot s_{\beta} \\
% & \geq \pis_{i,j} \cdot v_{i,j} \cdot s_{\beta},
% \end{align*}
% where $s_{\beta} = m_{\beta} + \frac{1 - m_{\beta}}{\beta}$.

% Proceeding as in the proof of Theorem~\ref{thm:rfpa_uniform_ub}, we conclude that PoA $\le 1.5$ when $\alpha=7.63$ and $\eta = 0.33$.
% \end{proof}
